# Supplementary material for: OpenWAM: An Open Framework for Composable World-Action Models
Source: arXiv:2610.07922 source file (2026-10-06)
Supplement: Supplementary file 1 [file a_results.tex]

\section{More Studies and Results}
\label{appendix:more_studies}
\subsection{Additional Case Studies}

To better understand how Vision-Language Models (VLMs) solve kinematic inference tasks beyond aggregate scores, we conduct a qualitative case study on the top-performing model, ChatGPT-5.1, using its \texttt{Thinking} mode in the standard user-facing interface.
For each selected video–text pair, we repeatedly query the model and inspect the tool-augmented chain-of-thought until we obtain representative traces that are syntactically well-formed and numerically valid.\footnote{We prompt the model multiple times and observe substantial variability: on the same instance, some runs produce accurate and well-structured reasoning, while others fail to parse the question or ignore key inputs.
We therefore collect several responses per instance and manually select representative traces that are syntactically coherent and numerically valid for detailed analysis.
A similar instability is also present in our API-based evaluation, even with temperature fixed to $0$; in the main benchmark, we address this by running multiple trials and recording a failure rate.}
We then analyze both the final numerical answers and the intermediate reasoning steps.\footnote{We emphasize that this analysis is diagnostic rather than evaluative: we study one specific model’s internal behavior to illustrate broader patterns of (un)faithful quantitative reasoning.}


Overall, we observe a sharp contrast between successful instances, where the model follows a textbook-like “measure pixels $\rightarrow$ apply prior $\rightarrow$ compute target” pipeline,  and failure modes, where it largely ignores the video and the provided prior, and instead falls back to pre-trained world knowledge or generic heuristics.
Below we discuss four representative cases.

\noindent\textbf{Case 1: Faithful pixel–prior reasoning.}
\autoref{fig:case1} shows a 2D scene with a yellow car moving laterally.
The model is asked two questions: (i) given that the car’s length is $5.67$\,m, what is its speed at $2.0$\,s; and (ii) what is the car’s width in meters.
In this instance, ChatGPT-5.1’s chain-of-thought closely matches the intended reasoning procedure.
The model first identifies the relevant frames around $t=2.0$\,s, uses OpenCV-style tools to obtain bounding boxes, and explicitly treats the longer side of the box (135\,px) as the car’s length in pixel space.
It then calibrates a pixel-to-meter scale from the given length prior (5.67\,m), and computes the width as
\[
\text{width} \approx \frac{58}{135} \times 5.67\text{m}\approx 2.44\text{m}\,,
\]
 which is close to the ground truth width and achieves high relative accuracy.
Here the model behaves as an input-faithful visual measurer: it grounds both the prior and the kinematic target in pixel space and performs the correct proportional reasoning.
When this pipeline is followed, the resulting numerical answers are often near the ground truth.

\begin{figure}
    \centering
    \includegraphics[width=0.99\linewidth]{sec/images/case1.pdf}
    \vspace{-0.5em}
    \caption{\textbf{Case 1: Faithful pixel–prior reasoning.}}
    \label{fig:case1}
\end{figure}

\noindent\textbf{Case 2: Counterfactual prior breaks faithfulness.}
In the second case (\autoref{fig:case2}), we reuse the same video but multiply the car-length prior by a counterfactual factor of 1000, changing the input to “length of the yellow car = 5670\,m.”
The task is again to infer speed at $2.0$\,s and the car’s width.
In its \texttt{Thinking} trace, the model explicitly notes that “5670\,m” is an implausible car length and expresses confusion.
Crucially, instead of continuing to rely on pixel measurements and the (counterfactual) prior, it effectively abandons the video and the numeric input.
For the width question, it switches to a generic heuristic, assuming a “typical car’s width-to-length ratio” and hallucinating a plausible-looking width independent of the actual scene.
The final width prediction happens to have high relative accuracy (close to $0.9$), but this success is not input-faithful; it arises from pre-trained knowledge about cars rather than from the specific video or the given prior.
This case highlights a key risk that purely outcome-based metrics can judge an answer as “good,” while the underlying reasoning ignores the provided evidence.

\begin{figure}
    \centering
    \includegraphics[width=0.99\linewidth]{sec/images/case2.pdf}
    \vspace{-0.5em}
    \caption{\textbf{Case 2: Counterfactual prior breaks faithfulness.}}
    \label{fig:case2}
\end{figure}

\noindent\textbf{Case 3: Video ablation reveals reliance on priors.}
Case 3 (\autoref{fig:case3}) uses a video-ablation setting. The model receives only the text prompt (including “length of the yellow car = 5.67\,m”), without access to the video.
When asked for the car’s speed at $2.0$\,s, ChatGPT-5.1 produces an answer ($12$\,m/s) that is far from the ground truth, confirming that motion estimation is difficult without visual evidence.
However, when asked for the car’s width (still without video), the model outputs a numerically reasonable value with relatively high accuracy (relative accuracy $\approx 0.7$).
Since no pixel information is available in this ablated setting, this behavior can only be explained by the model’s internal prior over typical car dimensions.
Combined with Case 1 and 2, this suggests a pattern that even when video is available, much of the “size” inference can be driven by pre-trained world knowledge rather than by explicit pixel measurements.

\begin{figure}
    \centering
    \includegraphics[width=0.99\linewidth]{sec/images/case3.pdf}
    \vspace{-0.5em}
    \caption{\textbf{Case 3: Video ablation reveals reliance on priors.}}
    \label{fig:case3}
\end{figure}

\noindent\textbf{Case 4: Strong gravitational prior overrides counterfactual physics.}
The fourth case (\autoref{fig:case4}) involves a Blender-simulated basketball scene that visually resembles a realistic indoor court, but with counterfactual physics. The ball’s acceleration is time-varying and close to $1\,\text{m/s}^2$, rather than standard gravity. The model is asked for the ball’s acceleration at $0.5$\,s and its speed at $1.5$\,s, given the ball’s diameter as a prior.
Here, ChatGPT-5.1 completely ignores both the video and the non-standard trajectory implied by the simulation.
It directly outputs the canonical gravitational acceleration $9.8\,\text{m/s}^2$, and for speed simply multiplies $g$ by time (i.e., $9.8 \times 1.5 = 14.7\,\text{m/s}$), leading to relative accuracy equals to $0$ on both queries.
No pixel measurements or scale computations appear in the \texttt{Thinking} trace.
This illustrates how strong pre-trained physical priors (e.g., “objects fall with acceleration $g$”) can dominate the model’s behavior, even when they contradict the actual visual input and the provided prior.

\begin{figure}
    \centering
    \includegraphics[width=0.99\linewidth]{sec/images/case4.pdf}
    \vspace{-0.5em}
    \caption{\textbf{Case 4: Strong gravitational prior overrides counterfactual physics.}}
    \label{fig:case4}
\end{figure}

\noindent\textbf{Discussion.}
These four cases collectively sharpen our main quantitative findings.
\begin{itemize}[leftmargin=*]
  \item When everything works, ChatGPT-5.1 can execute an impressive, tool-augmented pipeline that does read pixel trajectories, apply the physical prior, and compute accurate kinematic quantities.
  \item However, this behavior is fragile. As soon as the prior becomes counterfactual, the video is ignored, or the underlying physics departs from familiar regimes, the model quickly reverts to pre-trained world knowledge or rough heuristics, often ignoring the provided inputs.
  \item High numerical accuracy does not guarantee input-faithful reasoning. Specifically, Case 2 demonstrates that a model can get the “right” answer for the wrong reasons, while Cases 3 \& 4 show that it can stick to canonical physical constants even when the scene violates them.
\end{itemize}

These observations suggest that improving VLMs’ quantitative physical reasoning will require not only better aggregate performance, but also mechanisms that encourage faithful use of visual evidence and explicit numerical priors, rather than letting powerful, but sometimes misleading, pre-trained world knowledge dominate the inference process.

\subsection{Metric Design Justification}
\label{appendix:metric_design}

In \textsc{QuantiPhy}, we adopt Mean Relative Accuracy (MRA) as the primary evaluation metric for quantitative physical inference tasks with continuous outputs.
Each prediction $\hat{y}$ is compared to the ground truth $y$ using its relative error $|\hat{y} - y| / y$, and awarded partial credit if the error falls below confidence thresholds $\theta \in \{0.5, 0.55, \ldots, 0.95\}$.
The final MRA score is the average of binary accuracies across these thresholds
\begin{equation}
\mathrm{MRA} = \frac{1}{10} \sum_{\theta \in \mathcal{C}}
\mathbbm{1} \left( \frac{|\hat{y} - y|}{|y|} < 1 - \theta \right),
\end{equation}
where $C = \{0.5, 0.55, \ldots, 0.95\}$ is the set of confidence thresholds.

While one could alternatively compute continuous relative error (e.g., mean relative error or mean absolute percentage error), we prefer MRA for several practical and conceptual reasons.

\noindent\textbf{Discrete but calibrated.}
MRA discretizes accuracy into a finite set of thresholds, offering interpretable feedback on how often the model is ``close enough'' under increasing demands.
Rather than penalizing deviations proportionally (which can be dominated by outliers), MRA provides a graded scale of correctness, similar in spirit to the mAP@IoU\footnote{mAP@IoU: Mean Average Precision (mAP) calculated at specific Intersection over Union (IoU) thresholds.} metrics in object detection.

\noindent\textbf{Robust to ambiguity and noise.}
Many video-based physical inferences involve semantic or visual uncertainty.
For example, estimating a person’s height may vary depending on whether hair or shoes are included;
estimating a cup’s diameter may depend on whether the inner or outer rim is used.
MRA tolerates such ambiguity by granting full credit when answers fall within a reasonable margin.

Moreover, measurement noise is often unavoidable:
\begin{itemize}
  \item \textbf{Temporal aliasing:} limited frame rates restrict temporal resolution for computing velocities and accelerations;
  \item \textbf{Motion blur:} fast-moving objects introduce visual uncertainty during measurement;
  \item \textbf{Imprecise priors:} even real-world scale references (e.g., credit card dimensions) may not be perfectly visible or aligned.
\end{itemize}
MRA accommodates these natural imperfections more flexibly than a regression-style loss.

\noindent\textbf{Supported by precedent.}
The MRA metric was introduced by Yang et al.~\cite{yang2025thinking} in VSI-Bench for evaluating numerical answers in visual–spatial reasoning tasks.
Some follow-up work~\cite{sridhar2025vreason, cai2025holistic} adopted the same evaluation to benchmark multimodal models in physical and spatial settings.
These works motivate MRA as a stable and discriminative way to capture proximity between predicted and ground-truth values, especially when scale varies across examples.
Our use of MRA continues this design choice, ensuring comparability while improving robustness.

In sum, MRA balances informativeness, robustness, and interpretability.
It is well-suited for evaluating VLMs on physically grounded, numerically sensitive tasks like those in \textsc{QuantiPhy}, where small deviations are acceptable, but large errors are unacceptable regardless of scale.



\begin{figure*}[ht!]
    \centering
    \includegraphics[width=0.80\linewidth]{sec/images/mra_density_plot.png}
    \caption{\textbf{Distribution of MRA by model.} One caveat to note is that the Avg. MRA in \autoref{tab:main-results} reflects the mean MRA across inference task categories for each model (i.e., the average MRA of \texttt{2D-Static}, \texttt{2D-Dynamic}, \texttt{3D-Static}, and \texttt{3D-Dynamic}). In contrast, the mean in this distribution plot represents the average MRA at the individual-question level for each model.}
    \label{fig:mra_density}
\end{figure*}

\subsection{Model MRA Distribution}

\autoref{fig:mra_density} visualizes the MRA distributions for each VLM. Each subplot shows a density curve with mean (gray solid) and median (blue dashed) lines, along with summary statistics (mean, std, median, Q25, Q75) displayed to the right.

The top-performing models, including ChatGPT-5.1, Gemini-2.5 Pro, Gemini-2.5 Flash, Qwen3-VL-instruct-32B, and Grok-4.1-Fast-Reasoning, show notably higher densities around moderate to high MRA values above 0.5, with means and medians clustering around 0.4–0.6. Their smoother, more concentrated curves indicate both higher accuracy and more consistent performance across the evaluation set.

A second tier of models, including InternVL-3.5-30B, Qwen3-VL-instruct-8B, Molmo-7B, and ChatGPT-5, exhibits slightly lower means and medians, generally around 0.3–0.4. Their broader distributions with heavier tails indicate greater variability that these models produce some strong outputs but also more low-scoring cases. The alignment of medians and means suggests errors are not extremely skewed.

Mid-tier models such as Qwen-3-VL-instruct-2B, Phi-4-Multimodal-Instruct, SmolVLM-Instruct, CogVLM2 Video, Claude-4.5 Sonnet, and VILA-7B show means of 0.2–0.3. Their distributions are heavily weighted toward low MRA values with thin right tails, indicating that while they occasionally achieve moderate scores, they rarely reach the performance levels of top-tier systems.

The weakest-performing models, for example, Phi-3-Mini-128K-Instruct-3.8B, LLaVA-13B, Fuyu-8B, and MiniCPM-V 4.5-8B, show distributions highly concentrated near zero. With means below 0.15 and medians around 0.0, these models fail to produce meaningful MRA performance in most cases.

Notably, many distributions have substantial mass centered around zero. An MRA of zero indicates either the model output zero as an answer or failed to produce proper numerical output. We also observed that some model APIs are unstable and produce errors over time, potentially due to API server error, running environment, internet traffic, batch size variations, etc. We abstract away from these in this paper and simply treat these failed cases as observations with MRA equal to zero.

Overall, modern frontier proprietary models cluster around substantially higher and more consistent MRA values, mid-tier models show moderate capability with noticeable variability, and smaller or older models yield predominantly low scores. The density patterns and comparative statistics reveal a clear performance gap between state-of-the-art systems and lightweight or earlier-generation models.
