# Supplementary material for: OpenWAM: An Open Framework for Composable World-Action Models
Source: arXiv:2610.07922 source file (2026-10-06)
Supplement: Supplementary file 6 [file g_assetcitation.tex]

\section{Sketchfab Model Sources}


In \autoref{tab:sketchfab_models}, we list the Model Name, Author, and Model ID for all Sketchfab models used in the Blender-generated videos in our dataset.
\onecolumn
\begin{longtable}{|p{6cm}|p{4cm}|p{6cm}|}
\caption{Sketchfab 3D Models} \label{tab:sketchfab_models} \\
\hline
\textbf{Model Name} & \textbf{Author} & \textbf{Model ID} \\
\hline
\endfirsthead

\multicolumn{3}{c}{\tablename\ \thetable\ -- \textit{Continued from previous page}} \\
\hline
\textbf{Model Name} & \textbf{Author} & \textbf{Model ID} \\
\hline
\endhead

\hline
\multicolumn{3}{r}{\textit{Continued on next page}} \\
\endfoot

\hline
\endlastfoot
Supermarket trolley broken & kreems & 7f460877380349f8886280a596253034 \\
\hline
supermarket 1 & amogusstrikesback2 & ca1def2b7be544068def3cec5852c67e \\
\hline
Pool Table (Animation) & Yanez Designs & 0f2ae181a2dd4b00a6ec25073692037f \\
\hline
Bowling Pack (Bowling Pins \& Ball) & EverZax & 52743c4714c14211ac71d2fe1e5c8da3 \\
\hline
Bowling Club & tiunov.se & 0b8fae45fcda4fe78f93bb2a899401a6 \\
\hline
Elephant & planeta-elefante & f8778fc3d161481abba7ec23a8ddd1e8 \\
\hline
Walking Astronaut & Unknown Animaker & d9062a2003df422abdafdc02afdac085 \\
\hline
Mr Man Walking & Instinto Ideal Studio & 98ccac2b0e2845789b6f789978ca06ed \\
\hline
Jupiter \& satellites & Sakado & 379fd77b970c4821898c05c483913dec \\
\hline
Model 92A - Great White Shark & DigitalLife3D & 702e7b53637f4ded9ca479a8124e810d \\
\hline
Model 95A - Adult Leatherback Sea Turtle, "Mac" & DigitalLife3D & 4974c93644a24da280fde68cba74a12d \\
\hline
Model 69A - Striped Bass & DigitalLife3D & 35be3af9a7c4441c98109e5562d36c09 \\
\hline
Underground Parking Lot & Janis Zeps & 0ad5c221525b4bbba3a164c6235d28b8 \\
\hline
Airport Car & Jungle Jim & 29d1c6260b134a3baf5231f34de1b24f \\
\hline
Airport Catering Truck & rwy00 & 289f4e2cfa3f4722b0476b1fc37681d8 \\
\hline
Towel & TheSpacePunk & 6edc341457e44603ab351470ab800493 \\
\hline
Plain Mug & LightSwitch & 19c8fe5702b544d0a1409d3dac1cf90e \\
\hline
Flour ARIDLL & fwild & d40db94d92ab4e7a82a1c199312f3985 \\
\hline
Milk & Multipainkiller Studio & 5e8d71045e2040ba8f6619d86d204cf5 \\
\hline
Apple [Scan] & hoxsvl.scan & facb1aa6928c4f8f82d87a019b9f134e \\
\hline
PACKAGING EMPAQUE DE HUEVOS & willinando1w08 & cd51c5d25bbd4370881aebd3648cfe8c \\
\hline
Kitchen Pack & GRIP420 & a513f2e85bc94ae5b6d8cbd74909e3c4 \\
\hline
Kitchen Tools & anybody & 417e3873fcb34f7ab9744506d7bcc838 \\
\hline
Coffee Shop Cup & David Zerba & 37e6805f2b7a4158a1d61fe75f8e2a33 \\
\hline
Cup & Dmytro Nikonov & 7d450bb714034fceaa7b59a0e564f46b \\
\hline
Bird Animations Alex & ahitch3 & 081fa7f0cfd649b9b07babb4c619acc7 \\
\hline
Dove Bird Rigged & FourthGreen & 6b91be2a28fb4404a2d57d5ca98bd4dc \\
\hline
POLICE CAR - Belgian VW Transporter & Mickael Boitte & 35eaf9505e13464385404402ad865508 \\
\hline
Jo on Bike - Rigged \& Animated & NEEEU Spaces GmbH & 36ee5344e81149858a664cde9f98e835 \\
\hline
Simple Factory Scene & Pickeri & 804fbe0cd1fa44fa9ca86ae42c82d63d \\
\hline
Car & Paulius & a619dd25a6c04af0b2d8730aa1cb058b \\
\hline
Basketball Court & tiunov.se & 5faad7b528124907ab82732ed0c6b743 \\
\hline
Basketball NBA Championship Official Trophy & johnnokomis & 04f6f1135ffb48749c43c9c20c75fc19 \\
\hline
Bouncing Basketball & Maurice Svay & b8731a2fda6849c9a164d1966dc16ff8 \\
\hline
Zen Japanese Tea House with Go Board & winters810 & a1e95e5efee349a693f30eda32401aef \\
\hline
Chinese Chess & chung\_the\_artist & 7ad0f4f0ebbc455d9e9f829c956dda80 \\
\hline
paper airplane & vesicalsnail & 0967ab4a9c654a569a13ea1f8d9dca0c \\
\hline
3d soccer ball & BlenderMaster & 0400146e0e3c4d8f8b57bfa06d7dfb4c \\
\hline
Cardboard Box & Pricey1600 & 4e622ef1a09c43e28a49d9fa37f9eeee \\
\hline
Tennis Ball Low-poly PBR & MaX3Dd & e5c2b0e5860549acaa2dfe8b764d5f94 \\
\hline
Old Camera Bag .::RAWscan::. & Andrea Spognetta (Spogna) & 788f8b75874f417ebde498ffd231410c \\
\hline
Animated ROBOT SDC & SDC PERFORMANCE & 3d127f327a6c4033a32b810b5fb071ed \\
\hline
Gift Box & local.yany & 83296611584143a3afad6c0d0c0a4227 \\
\hline
Sci-fi Box & Igor\_K. & ca415724f32043489fcab2ec74582619 \\
\hline
Cat Walk & LostBoyz2078 & 915680200c064815bba75e008ba9efb5 \\
\hline
Deer walk & LostBoyz2078 & 229ba6ba0d1e4811ab89382f74601e16 \\
\hline
Horse & kenchoo & 86d47bdcd5ab41238ba44547e4d21f9c \\
\hline
Horse Walk & Amitesh Nandan & 93b53ddcec414592842753d1819f3133 \\
\hline
Rabbit Rigged & FourthGreen & e7213589744d436b9d96e2dbb31198a5 \\
\hline
phoenix bird & NORBERTO-3D & 844ba0cf144a413ea92c779f18912042 \\
\hline
First Aid DX2 - 300 Followers Celebration & re1monsen & c5ddfa9e6309403083bbce60bdcc3d71 \\
\hline
Nathan Animated 003 - Walking 3D Man & Renderpeople & 143a2b1ea5eb4385ae90a73657aca3bc \\
\hline
Chernovan Nemesis & Swiss\_Fox & c6c91c73e93444f4b72d6c24db778e73 \\
\hline
Dragon Fly & LostBoyz2078 & 1443a7efe5d5450b8db4c15d8ff5c343 \\
\hline
Borboleta Azul - Butterfly & Lancaster Modelagem 3D & ab9192b6bc8f49e3baed63e984c7073a \\
\hline
Blue Whale - Textured & Bohdan Lvov & d24d19021c724c3a9134eebcb76b0e0f \\
\hline
jellyfish & yanix & d06a5a553fe641ab92f720527b2278f3 \\
\hline
Koi Fish & 7PLUS & 236859b809984f52b70c94fd040b9c59 \\
\hline
Running Raccoon Animation & Santrez & bfce4d4815234c39bcf012352e52c27e \\
\hline
(FREE) Cyberpunk Hovercar & Lionsharp Studios & 3205b1075bb44ffc826bce0c2a04d74c \\
\hline
White Eagle Animation Fast Fly & GremorySaiyan & 30203bf39e5145f19c79e83c550139d3 \\
\hline
\end{longtable}
